# Supplementary material for: Evaluation Metrics for Object Detection for Autonomous Systems
Source: arXiv:2210.10298 source file (2022-10-19)
Supplement: Supplementary file 1 [file appendix.tex]

\section{Appendix}
\subsection{Sensor: $CAM\_FRONT$}
\subsubsection{Proposition-based Confusion Matrix}
\begin{tabular}{|l|cccc|}
\hline
 \diagbox{\textit{Pred}}{\textit{True}} &   \textit{ped} &  \textit{obs} &   \textit{ped}, \textit{obs} &   \textit{empty} \\
\hline
\textit{ped}          &               6 &               0 &                           12 &            0 \\
 \textit{obs}              &                 0 &              19 &                            0 &            0 \\
 \textit{ped},\textit{obs} &                 0 &               0 &                            0 &            0 \\
 \textit{empty}                 &                11 &              46 &                            2 &          298 \\
\hline
\end{tabular}

\begin{tabular}{|l|cccc|}
\hline
\diagbox{\textit{Pred}}{\textit{True}} &   \textit{ped} &  \textit{obs} &   \textit{ped}, \textit{obs} &   \textit{empty} \\
\hline
\textit{ped}          &                12 &               0 &                            4 &            0 \\
 \textit{obs}              &                 0 &             117 &                           19 &            0 \\
 \textit{ped},\textit{obs} &                 0 &               0 &                            4 &            0 \\
 \textit{empty}                 &                41 &              68 &                           12 &          117 \\
\hline
\end{tabular}

\begin{tabular}{|l|cccc|}
\hline
 \diagbox{\textit{Pred}}{\textit{True}} &   \textit{ped} &  \textit{obs} &   \textit{ped}, \textit{obs} &   \textit{empty} \\
\hline
\textit{ped}          &                3 &               0 &                            8 &            0 \\
 \textit{obs}              &                 0 &             106 &                           34 &            0 \\
 \textit{ped},\textit{obs} &                 0 &               2 &                            9 &            0 \\
 \textit{empty}                 &                16 &             121 &                           25 &           70 \\
\hline
\end{tabular}

\begin{tabular}{|l|cccc|}
\hline
 \diagbox{\textit{Pred}}{\textit{True}} &   \textit{ped} &  \textit{obs} &   \textit{ped}, \textit{obs} &   \textit{empty} \\
\hline
\textit{ped}          &                 1 &               0 &                            2 &            0 \\
 \textit{obs}              &                 0 &              69 &                           19 &            0 \\
 \textit{ped},\textit{obs} &                 0 &               0 &                            3 &            0 \\
 \textit{empty}                 &                18 &             119 &                           28 &          135 \\

\hline
\end{tabular}

\begin{tabular}{|l|cccc|}
\hline
\diagbox{\textit{Pred}}{\textit{True}}&   \textit{ped} &  \textit{obs} &   \textit{ped}, \textit{obs} &   \textit{empty} \\
\hline
\textit{ped}          &                0 &               0 &                            0 &            0 \\
 \textit{obs}              &                 0 &              47 &                           15 &            0 \\
 \textit{ped},\textit{obs} &                 0 &               0 &                            0 &            0 \\
 \textit{empty}                 &                12 &             123 &                           17 &          180 \\
\hline
\end{tabular}

\begin{tabular}{|l|cccc|}
\hline
 \diagbox{\textit{Pred}}{\textit{True}} &   \textit{ped} &  \textit{obs} &   \textit{ped}, \textit{obs} &   \textit{empty} \\
\hline
\textit{ped}          &                0 &               0 &                            0 &            0 \\
 \textit{obs}              &                 0 &              23 &                           21 &            0 \\
 \textit{ped},\textit{obs} &                 0 &               0 &                            0 &            0 \\
 \textit{empty}                 &                10 &             128 &                           46 &          166 \\

\hline
\end{tabular}

\begin{tabular}{|l|cccc|}
\hline
 \diagbox{\textit{Pred}}{\textit{True}} &   \textit{ped} &  \textit{obs} &   \textit{ped}, \textit{obs} &   \textit{empty} \\
\hline
\textit{ped}          &                0 &               0 &                            0 &            0 \\
 \textit{obs}              &                 0 &              24 &                            3 &            0 \\
 \textit{ped},\textit{obs} &                 0 &               0 &                            0 &            0 \\
 \textit{empty}                 &                 7 &             134 &                           30 &          196 \\
\hline
\end{tabular}

\begin{tabular}{|l|cccc|}
\hline
\diagbox{\textit{Pred}}{\textit{True}} &   \textit{ped} &  \textit{obs} &   \textit{ped}, \textit{obs} &   \textit{empty} \\
\hline
\textit{ped}          &                0 &               0 &                            0 &            0 \\
 \textit{obs}              &                 0 &              15 &                            0 &            0 \\
 \textit{ped},\textit{obs} &                 0 &               0 &                            0 &            0 \\
 \textit{empty}                 &                32 &             114 &                            7 &          226 \\
\hline
\end{tabular}

\begin{tabular}{|l|cccc|}
\hline
\diagbox{\textit{Pred}}{\textit{True}}&   \textit{ped} &  \textit{obs} &   \textit{ped}, \textit{obs} &   \textit{empty} \\
\hline
\textit{ped}          &                 0 &               0 &                            0 &            0 \\
 \textit{obs}               &                 0 &               8 &                            1 &            0 \\
 \textit{ped}, \textit{obs} &                 0 &               0 &                            0 &            0 \\
 \textit{empty}                &                 9 &              78 &                            3 &          295 \\
\hline
\end{tabular}

\begin{tabular}{|l|cccc|}
\hline
\diagbox{\textit{Pred}}{\textit{True}}&   \textit{ped} &  \textit{obs} &   \textit{ped}, \textit{obs} &   \textit{empty} \\
\hline
\textit{ped}          &                 0 &               3 &                            0 &            0 \\
\textit{obs}            &                 0 &               0 &                            0 &            0 \\
 \textit{ped}, \textit{obs} &                 0 &               0 &                            0 &            0 \\
\textit{empty}               &                 6 &              37 &                            0 &          348 \\
\hline
\end{tabular}

\subsubsection{Class-based Confusion Matrix}
\begin{minipage}{.5\textwidth}
 \centering
  \caption{}
  \label{tab:cb_0_10}
\begin{tabular}{|l|rrr|}
\hline
\diagbox{\textit{Pred}}{\textit{True}}       &  \textit{ped} &  \textit{obs} &  \textit{emp} \\
\hline
\textit{ped} &                36 &               0 &            0 \\
\textit{obs}   &                 0 &              19 &            0 \\
\textit{emp}      &                54 &              73 &          298 \\
\hline
\end{tabular}
\end{minipage}

\begin{minipage}{.5\textwidth}
 \centering
  \caption{}
  \label{tab:cb_10_20} 
\begin{tabular}{|l|rrr|}
\hline
\diagbox{\textit{Pred}}{\textit{True}}   &  \textit{ped} &  \textit{obs} &  \textit{emp} \\
\hline
\textit{ped} &                26 &               0 &            0 \\
\textit{obs}   &                 0 &             185 &            0 \\
\textit{emp}      &               169 &             360 &          117 \\
\hline
\end{tabular}
\end{minipage}

\begin{minipage}{.5\textwidth}
 \centering
  \caption{}
  \label{tab:cb_20_30}
\begin{tabular}{|l|rrr|}
\hline
\diagbox{\textit{Pred}}{\textit{True}}   & \textit{ped} &  \textit{obs} &  \textit{emp} \\
\hline
\textit{ped} &                23 &               2 &            0 \\
\textit{obs}   &                 0 &             183 &            0 \\
\textit{emp}      &               264 &             770 &           70 \\
\hline
\end{tabular}
\end{minipage}

\begin{minipage}{.5\textwidth}
 \centering
  \caption{}
  \label{tab:cb_30_40}
\begin{tabular}{|l|rrr|}
\hline
\diagbox{\textit{Pred}}{\textit{True}} &  \textit{ped} &  \textit{obs} &  \textit{emp} \\
\hline
\textit{ped} &                 6 &               0 &            0 \\
\textit{obs}   &                 0 &             109 &            0 \\
\textit{emp}      &               177 &             620 &          135 \\
\hline
\end{tabular}
\end{minipage}

\begin{minipage}{.5\textwidth}
 \centering
  \caption{}
  \label{tab:cb_40_50} 
\begin{tabular}{|l|rrr|}
\hline
\diagbox{\textit{Pred}}{\textit{True}}  &  \textit{ped} &  \textit{obs} &  \textit{emp} \\
\hline
\textit{ped} &                 0 &               0 &            0 \\
\textit{obs}   &                 0 &              72 &            0 \\
\textit{emp}      &               104 &             450 &          180 \\
\hline
\end{tabular}
 \end{minipage}
 
\begin{minipage}{.5\textwidth}
 \centering
  \caption{}
  \label{tab:cb_50_60}
\begin{tabular}{|l|rrr|}
\hline
\diagbox{\textit{Pred}}{\textit{True}}&  \textit{ped} &  \textit{obs} &  \textit{emp} \\
\hline
\textit{ped} &                 0 &               0 &            0 \\
\textit{obs}   &                 0 &              57 &            0 \\
\textit{emp}      &               142 &             440 &          166 \\
\hline
\end{tabular}
 \end{minipage}
 
\begin{minipage}{.5\textwidth}
 \centering
  \caption{}
  \label{tab:cb_60_70}
\begin{tabular}{|l|rrr|}
\hline
\diagbox{\textit{Pred}}{\textit{True}} &  \textit{ped} &  \textit{obs} &  \textit{emp} \\
\hline
\textit{ped} &                 0 &               0 &            0 \\
\textit{obs}   &                 0 &              27 &            0 \\
\textit{emp}      &                67 &             341 &          196 \\
\hline
\end{tabular}
 \end{minipage}
 
 \begin{minipage}{.5\textwidth}
 \centering
  \caption{}
  \label{tab:cb_70_80}
\begin{tabular}{|l|rrr|}
\hline
\diagbox{\textit{Pred}}{\textit{True}}  &  \textit{ped} &  \textit{obs} &  \textit{emp} \\
\hline
\textit{ped} &                 0 &               0 &            0 \\
\textit{obs}   &                 0 &              15 &            0 \\
\textit{emp}      &                43 &             196 &          226 \\
\hline
\end{tabular}
 \end{minipage}
 
 \begin{minipage}{.5\textwidth}
 \centering
  \caption{}
  \label{tab:cb_80_90}
\begin{tabular}{|l|rrr|}
\hline
\diagbox{\textit{Pred}}{\textit{True}}  &  \textit{ped} &  \textit{obs} &  \textit{emp} \\
\hline
\textit{ped} &                 0 &               0 &            0 \\
\textit{obs}   &                 0 &               9 &            0 \\
\textit{emp}      &                13 &              95 &          295 \\
\hline
\end{tabular}
 \end{minipage}
 
 \begin{minipage}{.5\textwidth}
 \centering
  \caption{}
  \label{tab:cb_90_100}
 \begin{tabular}{|l|rrr|}
\hline
\diagbox{\textit{Pred}}{\textit{True}}   &  \textit{ped} &  \textit{obs} &  \textit{emp} \\
\hline
\textit{ped} &                 0 &               0 &            0 \\
\textit{obs}   &                 0 &               3 &            0 \\
\textit{emp}      &                 6 &              46 &          348 \\
\hline
\end{tabular}
\end{minipage}

\subsection{Sensor: $CAM\_FRONT\_LEFT$ sensor}
\subsubsection{Proposition-based CM}
\begin{tabular}{|l|rrrr|}
\hline
                            &  \textit{ped} &  \textit{obs} &   ('obstacle', 'pedestrian') &  \textit{emp} \\
\hline
\textit{ped}            &                11 &               0 &                            1 &            0 \\
\textit{obs}              &                 0 &              71 &                           12 &            0 \\
 ('obstacle', 'pedestrian') &                 0 &               0 &                            2 &            0 \\
\textit{emp}                 &                17 &              24 &                            2 &          254 \\
\hline
\end{tabular}
 
Printing confusion matrix from distance d <= 20.0
\begin{tabular}{|l|rrrr|}
\hline
                            &  \textit{ped} &  \textit{obs} &   ('obstacle', 'pedestrian') &  \textit{emp} \\
\hline
\textit{ped}            &                 9 &               0 &                           13 &            0 \\
\textit{obs}              &                 0 &              36 &                           25 &            0 \\
 ('obstacle', 'pedestrian') &                 0 &               0 &                            5 &            0 \\
\textit{emp}                 &                55 &              37 &                           20 &          194 \\
\hline
\end{tabular}
 
Printing confusion matrix from distance d <= 30.0
\begin{tabular}{|l|rrrr|}
\hline
                            &  \textit{ped} &  \textit{obs} &   ('obstacle', 'pedestrian') &  \textit{emp} \\
\hline
\textit{ped}            &                 1 &               0 &                            1 &            0 \\
\textit{obs}              &                 0 &              19 &                            8 &            0 \\
 ('obstacle', 'pedestrian') &                 0 &               0 &                            1 &            0 \\
\textit{emp}                 &                37 &              82 &                           19 &          226 \\
\hline
\end{tabular}
 
Printing confusion matrix from distance d <= 40.0
\begin{tabular}{|l|rrrr|}
\hline
                            &  \textit{ped} &  \textit{obs} &   ('obstacle', 'pedestrian') &  \textit{emp} \\
\hline
\textit{ped}            &                 0 &               0 &                            0 &            0 \\
\textit{obs}              &                 0 &              11 &                            0 &            0 \\
 ('obstacle', 'pedestrian') &                 0 &               0 &                            0 &            0 \\
\textit{emp}                 &                18 &              70 &                           13 &          282 \\
\hline
\end{tabular}
 
Printing confusion matrix from distance d <= 50.0
\begin{tabular}{|l|rrrr|}
\hline
                            &  \textit{ped} &  \textit{obs} &   ('obstacle', 'pedestrian') &  \textit{emp} \\
\hline
\textit{ped}            &                 0 &               0 &                            0 &            0 \\
\textit{obs}              &                 0 &               3 &                            1 &            0 \\
 ('obstacle', 'pedestrian') &                 0 &               0 &                            0 &            0 \\
\textit{emp}                 &                13 &              44 &                            2 &          331 \\
\hline
\end{tabular}
 
Printing confusion matrix from distance d <= 60.0
\begin{tabular}{|l|rrrr|}
\hline
                            &  \textit{ped} &  \textit{obs} &   ('obstacle', 'pedestrian') &  \textit{emp} \\
\hline
\textit{ped}            &                 0 &               0 &                            0 &            0 \\
\textit{obs}              &                 0 &               6 &                            0 &            0 \\
 ('obstacle', 'pedestrian') &                 0 &               0 &                            0 &            0 \\
\textit{emp}                 &                23 &              30 &                           11 &          324 \\
\hline
\end{tabular}
 
Printing confusion matrix from distance d <= 70.0
\begin{tabular}{|l|rrrr|}
\hline
                            &  \textit{ped} &  \textit{obs} &   ('obstacle', 'pedestrian') &  \textit{emp} \\
\hline
\textit{ped}            &                 0 &               0 &                            0 &            0 \\
\textit{obs}              &                 0 &               5 &                            4 &            0 \\
 ('obstacle', 'pedestrian') &                 0 &               0 &                            0 &            0 \\
\textit{emp}                 &                 1 &              16 &                           22 &          346 \\
\hline
\end{tabular}
 
Printing confusion matrix from distance d <= 80.0
\begin{tabular}{|l|rrrr|}
\hline
                            &  \textit{ped} &  \textit{obs} &   ('obstacle', 'pedestrian') &  \textit{emp} \\
\hline
\textit{ped}            &                 0 &               0 &                            0 &            0 \\
\textit{obs}              &                 0 &               0 &                            0 &            0 \\
 ('obstacle', 'pedestrian') &                 0 &               0 &                            0 &            0 \\
\textit{emp}                 &                 6 &              43 &                           12 &          333 \\
\hline
\end{tabular}
 
Printing confusion matrix from distance d <= 90.0
\begin{tabular}{|l|rrrr|}
\hline
                            &  \textit{ped} &  \textit{obs} &   ('obstacle', 'pedestrian') &  \textit{emp} \\
\hline
\textit{ped}            &                 0 &               0 &                            0 &            0 \\
\textit{obs}              &                 0 &               0 &                            0 &            0 \\
 ('obstacle', 'pedestrian') &                 0 &               0 &                            0 &            0 \\
\textit{emp}                 &                 0 &              33 &                            0 &          361 \\
\hline
\end{tabular}
 
Printing confusion matrix from distance d <= 100.0
\begin{tabular}{|l|rrrr|}
\hline
                            &  \textit{ped} &  \textit{obs} &   ('obstacle', 'pedestrian') &  \textit{emp} \\
\hline
\textit{ped}            &                 0 &               0 &                            0 &            0 \\
\textit{obs}              &                 0 &               0 &                            0 &            0 \\
 ('obstacle', 'pedestrian') &                 0 &               0 &                            0 &            0 \\
\textit{emp}                 &                 0 &               4 &                            0 &          390 \\
\hline
\end{tabular}

\subsubsection{Class-based CM}
\begin{minipage}{.5\textwidth}
 \centering
 \caption{}
 \label{tab:cb_fl_0_10}
\begin{tabular}{|l|rrr|}
\hline
\diagbox{\textit{Pred}}{\textit{True}}       &  \textit{ped} &  \textit{obs} &  \textit{emp} \\
\hline
\textit{ped} &                16 &               0 &            0 \\
\textit{obs}   &                 0 &              90 &            0 \\
\textit{emp}      &                62 &              55 &          254 \\
\hline
\end{tabular}
\end{minipage}

\begin{minipage}{.5\textwidth}
 \centering
  \caption{}
  \label{tab:cb_10_20} 
\begin{tabular}{|l|rrr|}
\hline
\diagbox{\textit{Pred}}{\textit{True}}   &  \textit{ped} &  \textit{obs} &  \textit{emp} \\
\hline
\textit{ped} &                41 &               0 &            0 \\
\textit{obs}   &                 0 &              86 &            0 \\
\textit{emp}      &               312 &             175 &          194 \\
\hline
\end{tabular}
\end{minipage}

\begin{minipage}{.5\textwidth}
 \centering
  \caption{}
  \label{tab:cb_fl_20_30}
\begin{tabular}{|l|rrr|}
\hline
\diagbox{\textit{Pred}}{\textit{True}}   & \textit{ped} &  \textit{obs} &  \textit{emp} \\
\hline
\textit{ped} &                 3 &               0 &            0 \\
\textit{obs}   &                 0 &              34 &            0 \\
\textit{emp}      &               144 &             214 &          226 \\
\hline
\end{tabular}
\end{minipage}

\begin{minipage}{.5\textwidth}
 \centering
  \caption{}
  \label{tab:cb_fl_30_40}
\begin{tabular}{|l|rrr|}
\hline
\diagbox{\textit{Pred}}{\textit{True}} &  \textit{ped} &  \textit{obs} &  \textit{emp} \\
\hline
\textit{ped} &                 0 &               0 &            0 \\
\textit{obs}   &                 0 &              11 &            0 \\
\textit{emp}      &                58 &             141 &          282 \\
\hline
\end{tabular}
\end{minipage}

\begin{minipage}{.5\textwidth}
 \centering
  \caption{}
  \label{tab:cb_fl_40_50} 
\begin{tabular}{|l|rrr|}
\hline
\diagbox{\textit{Pred}}{\textit{True}}  &  \textit{ped} &  \textit{obs} &  \textit{emp} \\
\hline
\textit{ped} &                 0 &               0 &            0 \\
\textit{obs}   &                 0 &               4 &            0 \\
\textit{emp}      &                27 &              89 &          331 \\
\hline
\end{tabular}
 \end{minipage}
 
\begin{minipage}{.5\textwidth}
 \centering
  \caption{}
  \label{tab:cb_fl_50_60}
\begin{tabular}{|l|rrr|}
\hline
\diagbox{\textit{Pred}}{\textit{True}}&  \textit{ped} &  \textit{obs} &  \textit{emp} \\
\hline
\textit{ped} &                 0 &               0 &            0 \\
\textit{obs}   &                 0 &               6 &            0 \\
\textit{emp}      &                41 &              52 &          324 \\
\hline
\end{tabular}
 \end{minipage}
 
\begin{minipage}{.5\textwidth}
 \centering
  \caption{}
  \label{tab:cb_fl_60_70}
\begin{tabular}{|l|rrr|}
\hline
\diagbox{\textit{Pred}}{\textit{True}} &  \textit{ped} &  \textit{obs} &  \textit{emp} \\
\hline
\textit{ped} &                 0 &               0 &            0 \\
\textit{obs}   &                 0 &               9 &            0 \\
\textit{emp}      &                42 &              65 &          346 \\
\hline
\end{tabular}
 \end{minipage}
 
 \begin{minipage}{.5\textwidth}
 \centering
  \caption{}
  \label{tab:cb_fl_70_80}
\begin{tabular}{|l|rrr|}
\hline
\diagbox{\textit{Pred}}{\textit{True}}  &  \textit{ped} &  \textit{obs} &  \textit{emp} \\
\hline
\textit{ped} &                 0 &               0 &            0 \\
\textit{obs}   &                 0 &               0 &            0 \\
\textit{emp}      &                18 &              56 &          333 \\
\hline
\end{tabular}
 \end{minipage}
 
 \begin{minipage}{.5\textwidth}
 \centering
  \caption{}
  \label{tab:cb_fl_80_90}
\begin{tabular}{|l|rrr|}
\hline
\diagbox{\textit{Pred}}{\textit{True}}  &  \textit{ped} &  \textit{obs} &  \textit{emp} \\
\hline
\textit{ped} &                 0 &               0 &            0 \\
\textit{obs}   &                 0 &               0 &            0 \\
\textit{emp}      &                 0 &              33 &          361 \\
\hline
\end{tabular}
 \end{minipage}
 
 \begin{minipage}{.5\textwidth}
 \centering
  \caption{}
  \label{tab:cb_fl_90_100}
 \begin{tabular}{|l|rrr|}
\hline
\diagbox{\textit{Pred}}{\textit{True}}   &  \textit{ped} &  \textit{obs} &  \textit{emp} \\
\hline
\textit{ped} &                 0 &               0 &            0 \\
\textit{obs}   &                 0 &               0 &            0 \\
\textit{emp}      &                 0 &               4 &          390 \\
\hline
\end{tabular}
\end{minipage}

\subsection{Sensor: $CAM\_FRONT\_RIGHT$ sensor}
\subsubsection{Proposition based CM}
\begin{minipage}{.5\textwidth}
 \centering
 \caption{}
 \label{tab:cb_fl_0_10}
\begin{tabular}{|l|rrrr|}
\hline
\diagbox{\textit{Pred}}{\textit{True}}       &  \textit{ped} &  \textit{obs} &   ('obstacle', 'pedestrian') &  \textit{emp} \\
\hline
\textit{ped}            &                 8 &               0 &                            1 &            0 \\
\textit{obs}              &                 0 &              58 &                            4 &            0 \\
 ('obstacle', 'pedestrian') &                 0 &               0 &                            0 &            0 \\
\textit{emp}                 &                17 &              55 &                            5 &          246 \\
\hline
\end{tabular}
\end{minipage}

\begin{minipage}{.5\textwidth}
 \centering
  \caption{}
  \label{tab:cb_10_20} 
\begin{tabular}{|l|rrrr|}
\hline
\diagbox{\textit{Pred}}{\textit{True}}   & \textit{ped} &  \textit{obs} &   ('obstacle', 'pedestrian') &  \textit{emp} \\
\hline
\textit{ped}            &                 3 &               1 &                            7 &            0 \\
\textit{obs}              &                 0 &             116 &                           20 &            0 \\
 ('obstacle', 'pedestrian') &                 0 &               0 &                            1 &            0 \\
\textit{emp}                 &                47 &              96 &                           16 &           87 \\
\hline
\end{tabular}
\end{minipage}

\begin{minipage}{.5\textwidth}
 \centering
  \caption{}
  \label{tab:cb_fl_20_30}
\begin{tabular}{|l|rrrr|}
\hline
\diagbox{\textit{Pred}}{\textit{True}}   & \textit{ped} &  \textit{obs} &   ('obstacle', 'pedestrian') &  \textit{emp} \\
\hline
\textit{ped}            &                 0 &               0 &                            6 &            0 \\
\textit{obs}              &                 0 &             107 &                           38 &            0 \\
 ('obstacle', 'pedestrian') &                 0 &               0 &                            3 &            0 \\
\textit{emp}                 &                15 &             116 &                           32 &           77 \\
\hline
\end{tabular}
\end{minipage}

\begin{minipage}{.5\textwidth}
 \centering
  \caption{}
  \label{tab:cb_fl_30_40}
\begin{tabular}{|l|rrrr|}
\hline
\diagbox{\textit{Pred}}{\textit{True}} &  \textit{ped} &  \textit{obs} &   ('obstacle', 'pedestrian') &  \textit{emp} \\
\hline
\textit{ped}            &                 2 &               0 &                            3 &            0 \\
\textit{obs}              &                 0 &              55 &                            1 &            0 \\
 ('obstacle', 'pedestrian') &                 0 &               0 &                            0 &            0 \\
\textit{emp}                 &                20 &             129 &                           21 &          163 \\
\hline
\end{tabular}
\end{minipage}

\begin{minipage}{.5\textwidth}
 \centering
  \caption{}
  \label{tab:pb_fr_40_50} 
\begin{tabular}{|l|rrrr|}
\hline
\diagbox{\textit{Pred}}{\textit{True}}  &  \textit{ped} &  \textit{obs} &   ('obstacle', 'pedestrian') &  \textit{emp} \\
\hline
\textit{ped}            &                 0 &               0 &                            0 &            0 \\
\textit{obs}              &                 0 &              27 &                            3 &            0 \\
 ('obstacle', 'pedestrian') &                 0 &               0 &                            0 &            0 \\
\textit{emp}                 &                17 &              99 &                           15 &          233 \\
 \hline
\end{tabular}
 \end{minipage}
 
\begin{minipage}{.5\textwidth}
 \centering
  \caption{}
  \label{tab:pb_fr_50_60}
\begin{tabular}{|l|rrrr|}
\hline
\diagbox{\textit{Pred}}{\textit{True}}&  \textit{ped} &  \textit{obs} &   ('obstacle', 'pedestrian') &  \textit{emp} \\
\hline
\textit{ped}            &                 0 &               0 &                            0 &            0 \\
\textit{obs}              &                 0 &               5 &                            4 &            0 \\
 ('obstacle', 'pedestrian') &                 0 &               0 &                            0 &            0 \\
\textit{emp}                 &                 3 &              89 &                            5 &          288 \\
\hline
\end{tabular}
 \end{minipage}
 
\begin{minipage}{.5\textwidth}
 \centering
  \caption{}
  \label{tab:pb_fr_60_70}
\begin{tabular}{|l|rrrr|}
\hline
\diagbox{\textit{Pred}}{\textit{True}} & \textit{ped} &  \textit{obs} &   ('obstacle', 'pedestrian') &  \textit{emp} \\
\hline
\textit{ped}            &                 0 &               0 &                            0 &            0 \\
\textit{obs}              &                 0 &               3 &                            1 &            0 \\
 ('obstacle', 'pedestrian') &                 0 &               0 &                            0 &            0 \\
\textit{emp}                 &                 1 &              62 &                            1 &          326 \\
\hline
\end{tabular}
 \end{minipage}
 
 \begin{minipage}{.5\textwidth}
 \centering
  \caption{}
  \label{tab:pb_fr_70_80}
\begin{tabular}{|l|rrrr|}
\hline
\diagbox{\textit{Pred}}{\textit{True}}  &  \textit{ped} &  \textit{obs} &   ('obstacle', 'pedestrian') &  \textit{emp} \\
\hline
\textit{ped}            &                 0 &               0 &                            0 &            0 \\
\textit{obs}              &                 0 &               0 &                            0 &            0 \\
 ('obstacle', 'pedestrian') &                 0 &               0 &                            0 &            0 \\
\textit{emp}                 &                 0 &              23 &                            0 &          371 \\
 \hline
\end{tabular}
 \end{minipage}
 
 \begin{minipage}{.5\textwidth}
 \centering
  \caption{}
  \label{tab:pb_fr_80_90}
\begin{tabular}{|l|rrrr|}
\hline
\diagbox{\textit{Pred}}{\textit{True}}  &  \textit{ped} &  \textit{obs} &   ('obstacle', 'pedestrian') &  \textit{emp} \\
\hline
\textit{ped}            &                 0 &               0 &                            0 &            0 \\
\textit{obs}              &                 0 &               0 &                            0 &            0 \\
 ('obstacle', 'pedestrian') &                 0 &               0 &                            0 &            0 \\
\textit{emp}                 &                 0 &               9 &                            0 &          385 \\
\hline
\end{tabular}
 \end{minipage}
 
 \begin{minipage}{.5\textwidth}
 \centering
  \caption{}
  \label{tab:pb_fr_90_100}
 \begin{tabular}{|l|rrrr|}
\hline
\diagbox{\textit{Pred}}{\textit{True}}   & \textit{ped} &  \textit{obs} &   ('obstacle', 'pedestrian') &  \textit{emp} \\
\hline
\textit{ped}            &                 0 &               0 &                            0 &            0 \\
\textit{obs}              &                 0 &               0 &                            0 &            0 \\
 ('obstacle', 'pedestrian') &                 0 &               0 &                            0 &            0 \\
\textit{emp}                 &                 0 &               0 &                            0 &          394 \\
\hline
\end{tabular}
\end{minipage}

\subsubsection{Class-based CM}
\begin{minipage}{.5\textwidth}
 \centering
 \caption{}
 \label{tab:cb_fr_0_10}
\begin{tabular}{|l|rrr|}
\hline
\diagbox{\textit{Pred}}{\textit{True}}       &  \textit{ped} &  \textit{obs} &  \textit{emp} \\
\hline
\textit{ped} &                10 &               0 &            0 \\
\textit{obs}   &                 0 &              70 &            0 \\
\textit{emp}      &                44 &             134 &          246 \\
\hline
\end{tabular}
\end{minipage}

\begin{minipage}{.5\textwidth}
 \centering
  \caption{}
  \label{tab:cb_fr_10_20} 
\begin{tabular}{|l|rrr|}
\hline
\diagbox{\textit{Pred}}{\textit{True}}   & \textit{ped} &  \textit{obs} &  \textit{emp} \\
\hline
\textit{ped} &                12 &               2 &            0 \\
\textit{obs}   &                 0 &             174 &            0 \\
\textit{emp}      &               211 &             617 &           87 \\
\hline
\end{tabular}
\end{minipage}

\begin{minipage}{.5\textwidth}
 \centering
  \caption{}
  \label{tab:cb_fr_20_30}
\begin{tabular}{|l|rrr|}
\hline
\diagbox{\textit{Pred}}{\textit{True}}   & \textit{ped} &  \textit{obs} &  \textit{emp} \\
\hline
\textit{ped} &                12 &               0 &            0 \\
\textit{obs}   &                 0 &             198 &            0 \\
\textit{emp}      &               326 &             670 &           77 \\
\hline
\end{tabular}
\end{minipage}

\begin{minipage}{.5\textwidth}
 \centering
  \caption{}
  \label{tab:cb_fr_30_40}
\begin{tabular}{|l|rrr|}
\hline
\diagbox{\textit{Pred}}{\textit{True}} &  \textit{ped} &  \textit{obs} &  \textit{emp} \\
\hline
\textit{ped} &                 5 &               0 &            0 \\
\textit{obs}   &                 0 &              64 &            0 \\
\textit{emp}      &               173 &             437 &          163 \\
\hline
\end{tabular}
\end{minipage}

\begin{minipage}{.5\textwidth}
 \centering
  \caption{}
  \label{tab:cb_fr_40_50} 
\begin{tabular}{|l|rrr|}
\hline
\diagbox{\textit{Pred}}{\textit{True}}  &  \textit{ped} &  \textit{obs} &  \textit{emp} \\
\hline
\textit{ped} &                 0 &               0 &            0 \\
\textit{obs}   &                 0 &              30 &            0 \\
\textit{emp}      &                83 &             342 &          233 \\
\hline
\end{tabular}
 \end{minipage}
 
\begin{minipage}{.5\textwidth}
 \centering
  \caption{}
  \label{tab:cb_fr_50_60}
\begin{tabular}{|l|rrr|}
\hline
\diagbox{\textit{Pred}}{\textit{True}}&  \textit{ped} &  \textit{obs} &  \textit{emp} \\
\hline
\textit{ped} &                 0 &               0 &            0 \\
\textit{obs}   &                 0 &              11 &            0 \\
\textit{emp}      &                17 &             195 &          288 \\
\hline
\end{tabular}
 \end{minipage}
 
\begin{minipage}{.5\textwidth}
 \centering
  \caption{}
  \label{tab:cb_fr_60_70}
\begin{tabular}{|l|rrr|}
\hline
\diagbox{\textit{Pred}}{\textit{True}} &  \textit{ped} &  \textit{obs} &  \textit{emp} \\
\hline
\textit{ped} &                 0 &               0 &            0 \\
\textit{obs}   &                 0 &               4 &            0 \\
\textit{emp}      &                 3 &             107 &          326 \\
\hline
\end{tabular}
 \end{minipage}
 
 \begin{minipage}{.5\textwidth}
 \centering
  \caption{}
  \label{tab:cb_fr_70_80}
\begin{tabular}{|l|rrr|}
\hline
\diagbox{\textit{Pred}}{\textit{True}}  &  \textit{ped} &  \textit{obs} &  \textit{emp} \\
\hline
\textit{ped} &                 0 &               0 &            0 \\
\textit{obs}   &                 0 &               0 &            0 \\
\textit{emp}      &                 0 &              43 &          371 \\
\hline
\end{tabular}
 \end{minipage}
 
 \begin{minipage}{.5\textwidth}
 \centering
  \caption{}
  \label{tab:cb_fr_80_90}
\begin{tabular}{|l|rrr|}
\hline
\diagbox{\textit{Pred}}{\textit{True}}  & \textit{ped} &  \textit{obs} &  \textit{emp} \\
\hline
\textit{ped} &                 0 &               0 &            0 \\
\textit{obs}   &                 0 &               0 &            0 \\
\textit{emp}      &                 0 &               9 &          385 \\
\hline
\end{tabular}
 \end{minipage}
 
 \begin{minipage}{.5\textwidth}
 \centering
  \caption{}
  \label{tab:cb_fr_90_100}
 \begin{tabular}{|l|rrr|}
\hline
\diagbox{\textit{Pred}}{\textit{True}}   &  \textit{ped} &  \textit{obs} &  \textit{emp} \\
\hline
\textit{ped} &                 0 &               0 &            0 \\
\textit{obs}   &                 0 &               0 &            0 \\
\textit{emp}      &                 0 &               0 &          394 \\
\hline
\end{tabular}
\end{minipage}

\subsection{4 classes with sensor $CAM\_FRONT$}
\subsubsection{Proposition-based (Mini)}
\begin{minipage}{.5\textwidth}
 \centering
 \caption{}
 \label{tab:cb_fmini_four_classes_0_10}
\begin{tabular}{|l|rrrr|}
\hline
\diagbox{\textit{Pred}}{\textit{True}}       &  \textit{ped} &  \textit{obs} &   ('obstacle', 'pedestrian') &  \textit{emp} \\
\hline
\textit{ped}            &                 8 &               0 &                            1 &            0 \\
\textit{obs}              &                 0 &              58 &                            4 &            0 \\
 ('obstacle', 'pedestrian') &                 0 &               0 &                            0 &            0 \\
\textit{emp}                 &                17 &              55 &                            5 &          246 \\
\hline
\end{tabular}
\end{minipage}

\subsubsection{Proposition-based (Full)}
\begin{minipage}{.5\textwidth}
 \centering
 \caption{}
 \label{tab:cb_ffull_four_classes_0_10}
\begin{tabular}{|l|rrrr|}
\hline
\diagbox{\textit{Pred}}{\textit{True}}       &  \textit{ped} &  \textit{obs} &   ('obstacle', 'pedestrian') &  \textit{emp} \\
\hline
\textit{ped}            &                 8 &               0 &                            1 &            0 \\
\textit{obs}              &                 0 &              58 &                            4 &            0 \\
 ('obstacle', 'pedestrian') &                 0 &               0 &                            0 &            0 \\
\textit{emp}                 &                17 &              55 &                            5 &          246 \\
\hline
\end{tabular}
\end{minipage}

\subsubsection{Class-based (Mini)}
\begin{minipage}{.5\textwidth}
 \centering
 \caption{}
 \label{tab:cb_fmini_four_classes_0_10}
\begin{tabular}{|l|rrrr|}
\hline
\diagbox{\textit{Pred}}{\textit{True}}       &  \textit{ped} &  \textit{obs} &   ('obstacle', 'pedestrian') &  \textit{emp} \\
\hline
\textit{ped}            &                 8 &               0 &                            1 &            0 \\
\textit{obs}              &                 0 &              58 &                            4 &            0 \\
 ('obstacle', 'pedestrian') &                 0 &               0 &                            0 &            0 \\
\textit{emp}                 &                17 &              55 &                            5 &          246 \\
\hline
\end{tabular}
\end{minipage}

\subsubsection{Class-based (Full)}
\begin{minipage}{.5\textwidth}
 \centering
 \caption{}
 \label{tab:cb_ffull_four_classes_0_10}
\begin{tabular}{|l|rrrr|}
\hline
\diagbox{\textit{Pred}}{\textit{True}}       &  \textit{ped} &  \textit{obs} &   ('obstacle', 'pedestrian') &  \textit{emp} \\
\hline
\textit{ped}            &                 8 &               0 &                            1 &            0 \\
\textit{obs}              &                 0 &              58 &                            4 &            0 \\
 ('obstacle', 'pedestrian') &                 0 &               0 &                            0 &            0 \\
\textit{emp}                 &                17 &              55 &                            5 &          246 \\
\hline
\end{tabular}
\end{minipage}

\section{Confusion Matrix (proposition-based)}
Printing confusion matrix from distance d <= 10.0
\begin{tabular}{|l|rrrr|}
\hline
                            &  \textit{ped} &  \textit{obs} &   ('pedestrian', 'obstacle') &  \textit{emp} \\
\hline
\textit{ped}            &                22 &               0 &                            5 &            0 \\
\textit{obs}              &                 0 &             184 &                            4 &            0 \\
 ('pedestrian', 'obstacle') &                 0 &               0 &                            0 &            0 \\
\textit{emp}                 &                63 &             354 &                           13 &         3227 \\
\hline
\end{tabular}
 
Printing confusion matrix from distance d <= 20.0
\begin{tabular}{|l|rrrr|}
\hline
                            &  \textit{ped} &  \textit{obs} &   ('pedestrian', 'obstacle') &  \textit{emp} \\
\hline
\textit{ped}            &                52 &               2 &                           39 &            0 \\
\textit{obs}              &                 0 &             714 &                           92 &            0 \\
 ('pedestrian', 'obstacle') &                 0 &               0 &                           28 &            0 \\
\textit{emp}                 &               180 &             662 &                          134 &         1969 \\
\hline
\end{tabular}
 
Printing confusion matrix from distance d <= 30.0
\begin{tabular}{|l|rrrr|}
\hline
                            &  \textit{ped} &  \textit{obs} &   ('pedestrian', 'obstacle') &  \textit{emp} \\
\hline
\textit{ped}            &               117 &               4 &                           43 &            0 \\
\textit{obs}              &                 0 &             678 &                          178 &            0 \\
 ('pedestrian', 'obstacle') &                 0 &               0 &                           40 &            0 \\
\textit{emp}                 &               311 &             883 &                          231 &         1387 \\
\hline
\end{tabular}
 
Printing confusion matrix from distance d <= 40.0
\begin{tabular}{|l|rrrr|}
\hline
                            &  \textit{ped} &  \textit{obs} &   ('pedestrian', 'obstacle') &  \textit{emp} \\
\hline
\textit{ped}            &                47 &               5 &                           52 &            0 \\
\textit{obs}              &                 0 &             602 &                          193 &            0 \\
 ('pedestrian', 'obstacle') &                 0 &               0 &                           36 &            0 \\
\textit{emp}                 &               321 &             878 &                          264 &         1474 \\
\hline
\end{tabular}
 
Printing confusion matrix from distance d <= 50.0
\begin{tabular}{|l|rrrr|}
\hline
                            &  \textit{ped} &  \textit{obs} &   ('pedestrian', 'obstacle') &  \textit{emp} \\
\hline
\textit{ped}            &                21 &               3 &                            7 &            0 \\
\textit{obs}              &                 0 &             515 &                          142 &            0 \\
 ('pedestrian', 'obstacle') &                 0 &               0 &                            1 &            0 \\
\textit{emp}                 &               302 &             907 &                          241 &         1733 \\
\hline
\end{tabular}
 
Printing confusion matrix from distance d <= 60.0
\begin{tabular}{|l|rrrr|}
\hline
                            &  \textit{ped} &  \textit{obs} &   ('pedestrian', 'obstacle') &  \textit{emp} \\
\hline
\textit{ped}            &                 8 &               3 &                            2 &            0 \\
\textit{obs}              &                 0 &             332 &                           53 &            0 \\
 ('pedestrian', 'obstacle') &                 0 &               0 &                            0 &            0 \\
\textit{emp}                 &               251 &             838 &                          197 &         2188 \\
\hline
\end{tabular}
 
Printing confusion matrix from distance d <= 70.0
\begin{tabular}{|l|rrrr|}
\hline
                            &  \textit{ped} &  \textit{obs} &   ('pedestrian', 'obstacle') &  \textit{emp} \\
\hline
\textit{ped}            &                 4 &               3 &                            0 &            0 \\
\textit{obs}              &                 0 &             146 &                           15 &            0 \\
 ('pedestrian', 'obstacle') &                 0 &               0 &                            0 &            0 \\
\textit{emp}                 &               206 &             668 &                           88 &         2742 \\
\hline
\end{tabular}
 
Printing confusion matrix from distance d <= 80.0
\begin{tabular}{|l|rrrr|}
\hline
                            &  \textit{ped} &  \textit{obs} &   ('pedestrian', 'obstacle') &  \textit{emp} \\
\hline
\textit{ped}            &                 2 &               1 &                            0 &            0 \\
\textit{obs}              &                 0 &              79 &                            5 &            0 \\
 ('pedestrian', 'obstacle') &                 0 &               0 &                            0 &            0 \\
\textit{emp}                 &               136 &             541 &                           31 &         3077 \\
\hline
\end{tabular}
 
Printing confusion matrix from distance d <= 90.0
\begin{tabular}{|l|rrrr|}
\hline
                            &  \textit{ped} &  \textit{obs} &   ('pedestrian', 'obstacle') &  \textit{emp} \\
\hline
\textit{ped}            &                 1 &               0 &                            0 &            0 \\
\textit{obs}              &                 0 &              34 &                            2 &            0 \\
 ('pedestrian', 'obstacle') &                 0 &               0 &                            0 &            0 \\
\textit{emp}                 &                51 &             337 &                           11 &         3436 \\
\hline
\end{tabular}
 
Printing confusion matrix from distance d <= 100.0
\begin{tabular}{|l|rrrr|}
\hline
                            &  \textit{ped} &  \textit{obs} &   ('pedestrian', 'obstacle') &  \textit{emp} \\
\hline
\textit{ped}            &                 0 &               0 &                            0 &            0 \\
\textit{obs}              &                 0 &              12 &                            0 &            0 \\
 ('pedestrian', 'obstacle') &                 0 &               0 &                            0 &            0 \\
\textit{emp}                 &                23 &             180 &                            6 &         3651 \\
\hline
\end{tabular}

\clearpage
\section{Confusion Matrix (class-based)}
Printing confusion matrix from distance d <= 10.0
\begin{tabular}{|l|rrr|}
\hline
                 &  \textit{ped} &  \textit{obs} &  \textit{emp} \\
\hline
\textit{ped} &                31 &               0 &            0 \\
\textit{obs}   &                 0 &             191 &            0 \\
\textit{emp}      &               127 &             734 &         3227 \\
\hline
\end{tabular}
 
Printing confusion matrix from distance d <= 20.0
\begin{tabular}{|l|rrr|}
\hline
                 &  \textit{ped} &  \textit{obs} &  \textit{emp} \\
\hline
\textit{ped} &               158 &               2 &            0 \\
\textit{obs}   &                 1 &             998 &            0 \\
\textit{emp}      &               873 &            3526 &         1969 \\
\hline
\end{tabular}
 
Printing confusion matrix from distance d <= 30.0
\begin{tabular}{|l|rrr|}
\hline
                 &  \textit{ped} &  \textit{obs} &  \textit{emp} \\
\hline
\textit{ped} &               291 &               4 &            0 \\
\textit{obs}   &                 0 &            1052 &            0 \\
\textit{emp}      &              1794 &            4689 &         1387 \\
\hline
\end{tabular}
 
Printing confusion matrix from distance d <= 40.0
\begin{tabular}{|l|rrr|}
\hline
                 &  \textit{ped} &  \textit{obs} &  \textit{emp} \\
\hline
\textit{ped} &               183 &               5 &            0 \\
\textit{obs}   &                 0 &             983 &            0 \\
\textit{emp}      &              1913 &            4132 &         1474 \\
\hline
\end{tabular}
 
Printing confusion matrix from distance d <= 50.0
\begin{tabular}{|l|rrr|}
\hline
                 &  \textit{ped} &  \textit{obs} &  \textit{emp} \\
\hline
\textit{ped} &                30 &               3 &            0 \\
\textit{obs}   &                 0 &             759 &            0 \\
\textit{emp}      &              1396 &            3093 &         1733 \\
\hline
\end{tabular}
 
Printing confusion matrix from distance d <= 60.0
\begin{tabular}{|l|rrr|}
\hline
                 &  \textit{ped} &  \textit{obs} &  \textit{emp} \\
\hline
\textit{ped} &                10 &               3 &            0 \\
\textit{obs}   &                 0 &             409 &            0 \\
\textit{emp}      &               848 &            2151 &         2188 \\
\hline
\end{tabular}
 
Printing confusion matrix from distance d <= 70.0
\begin{tabular}{|l|rrr|}
\hline
                 &  \textit{ped} &  \textit{obs} &  \textit{emp} \\
\hline
\textit{ped} &                 5 &               3 &            0 \\
\textit{obs}   &                 0 &             171 &            0 \\
\textit{emp}      &               555 &            1167 &         2742 \\
\hline
\end{tabular}
 
Printing confusion matrix from distance d <= 80.0
\begin{tabular}{|l|rrr|}
\hline
                 &  \textit{ped} &  \textit{obs} &  \textit{emp} \\
\hline
\textit{ped} &                 2 &               1 &            0 \\
\textit{obs}   &                 0 &              85 &            0 \\
\textit{emp}      &               281 &             761 &         3077 \\
\hline
\end{tabular}
 
Printing confusion matrix from distance d <= 90.0
\begin{tabular}{|l|rrr|}
\hline
                 &  \textit{ped} &  \textit{obs} &  \textit{emp} \\
\hline
\textit{ped} &                 1 &               0 &            0 \\
\textit{obs}   &                 0 &              36 &            0 \\
\textit{emp}      &                88 &             409 &         3436 \\
\hline
\end{tabular}
\par
Printing confusion matrix from distance d <= 100.0
\begin{tabular}{|l|rrr|}
\hline
                 &  \textit{ped} &  \textit{obs} &  \textit{emp} \\
\hline
\textit{ped} &                 0 &               0 &            0 \\
\textit{obs}   &                 0 &              12 &            0 \\
\textit{emp}      &                35 &             207 &         3651 \\
\hline
\end{tabular}
